# Supplementary material for: Learning to detect RFI in radio astronomy without seeing it
Source: arXiv:2207.00351 source file (2022-10-11)
Supplement: Supplementary file 1 [file 7_Appendices.tex]

\appendix
\section{Appendix}
\label{sec:appendix}
